# Supplementary material for: From diamond to BC8 to simple cubic and back: kinetic pathways to post-diamond carbon phases from metadynamics
Source: arXiv:2509.00423 ancillary file (2025-08-30)
Supplement: Supplementary file 1 [file SupplementalMaterial.pdf]

# From diamond to BC8 to simple cubic and back: kinetic pathways to post-diamond carbon phases from metadynamics

## Supplemental Material

Roman Martoňák<sup>1</sup>, Sergey Galitskiy<sup>2</sup>, Azat O. Tipseev<sup>2</sup>, Joseph M. Gonzalez<sup>2</sup>, and Ivan I. Oleynik<sup>2</sup>

<sup>1</sup>*Department of Experimental Physics, Faculty of Mathematics, Physics and Informatics, Comenius University, Mlynská Dolina F2, 842 48 Bratislava, Slovakia*

<sup>2</sup>*University of South Florida, Tampa, Florida 33620, USA*

August 30, 2025

This Supplemental Material provides additional details supporting the results presented in the paper - description of the collective variables (CVs) employed in metadynamics, description of the NPT MD simulations, the parameters of metadynamics simulations, the graphs of CVs and time evolution of the fractions of structural phases, details and properties of the new *P222* structure, as well as details of the algorithm employed to identify the crystalline phases during the evolution of the system.

## Computational details - NPT MD, metadynamics and collective variables

In our metadynamics simulations we employed, similarly to Ref. [S1], mean coordination numbers as collective variables. The collective variables and metadynamics were implemented by using the PLUMED package [S2]. The mean coordination number is defined as follows

$$CN = \frac{2}{N} \sum_{i < j} s_{ij} \quad (1)$$

where  $N$  is the number of atoms and the switching function  $s_{ij}$  is defined as

$$s_{ij} = \frac{1}{1 + \left(\frac{r_{ij} - d_0}{r_0}\right)^6} \quad (2)$$

For more information see the documentation on the COORDINATION keyword [S2].

In Fig.S1 we show the radial distribution functions of the four relevant phases - cubic diamond, hexagonal diamond, BC8 and simple cubic at 1.5 TPa and 4000 K. The inflection points of the switching functions are located beyond the first and before the second coordination shell where the relevant phases differ significantly. The values of the parameters of the switching functions are listed below for each of the runs presented.

Variable-cell NPT molecular dynamics was performed by the LAMMPS package [S3] using the npt fix (for more information see the documentation [S3]). The time step was chosen as 1 fs. For temperature control we used thermostat with a time constant of 0.25 ps while for pressure control we use barostat with the time constant of 0.5 ps. We used the triclinic version of the barostat in order to sample both volume and shape fluctuations of the simulation supercell.

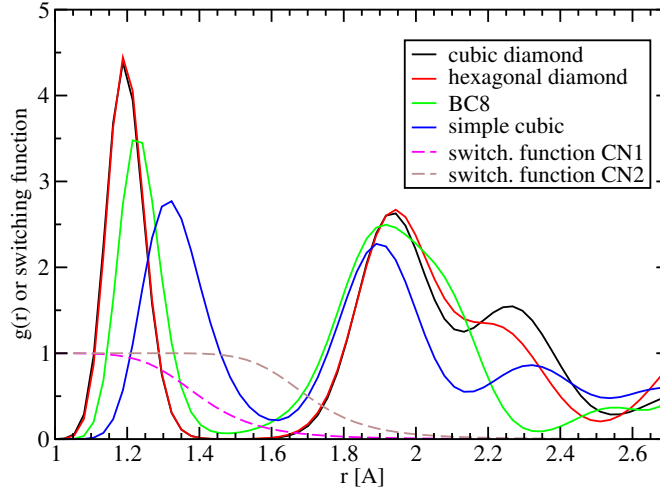

Fig.S1 Radial distribution functions for the four phases CD, HD, BC8, SC at 1.5 TPa and 4000 K. The switching functions defining collective variables CN1, CN2 are also shown.

## Transition from cubic diamond to BC8, 1.5 TPa and 4000 K

4096 atoms

CN1:  $D_0 = 0.09$  nm,  $R_0 = 0.05$  nm,  $\sigma = 0.02$

CN2:  $D_0 = 0.12$  nm,  $R_0 = 0.05$  nm,  $\sigma = 0.05$

$W = 300$  kJ/mol,  $PACE = 1000$

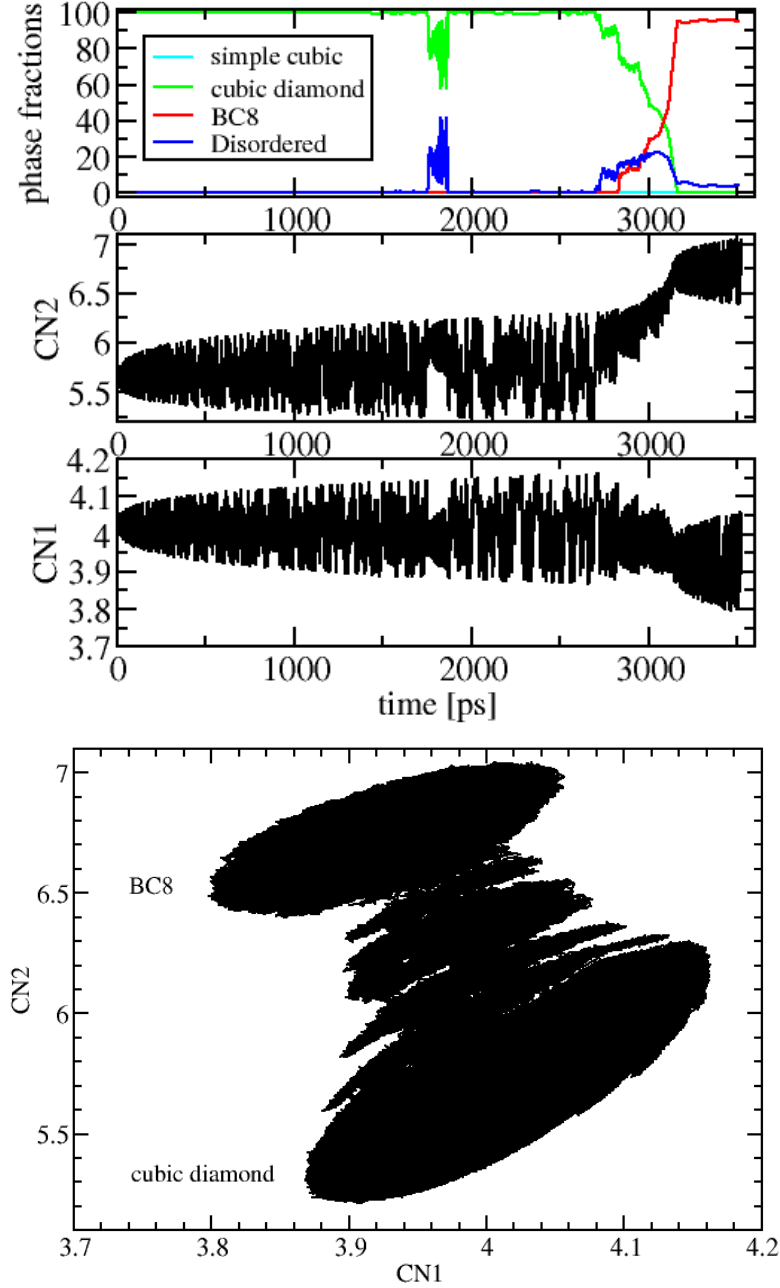

Fig.S2 Upper panel: time evolution of the collective variables  $CN1$  and  $CN2$  and phase fractions. Lower panel: Space of the CVs explored by metadynamics.

## Transition from cubic diamond to BC8, 1.8 TPa and 3000 K

4096 atoms

CN1:  $D_0 = 0.09$  nm,  $R_0 = 0.05$  nm,  $\sigma = 0.02$

CN2:  $D_0 = 0.12$  nm,  $R_0 = 0.05$  nm,  $\sigma = 0.05$

$W = 300$  kJ/mol,  $PACE = 1000$

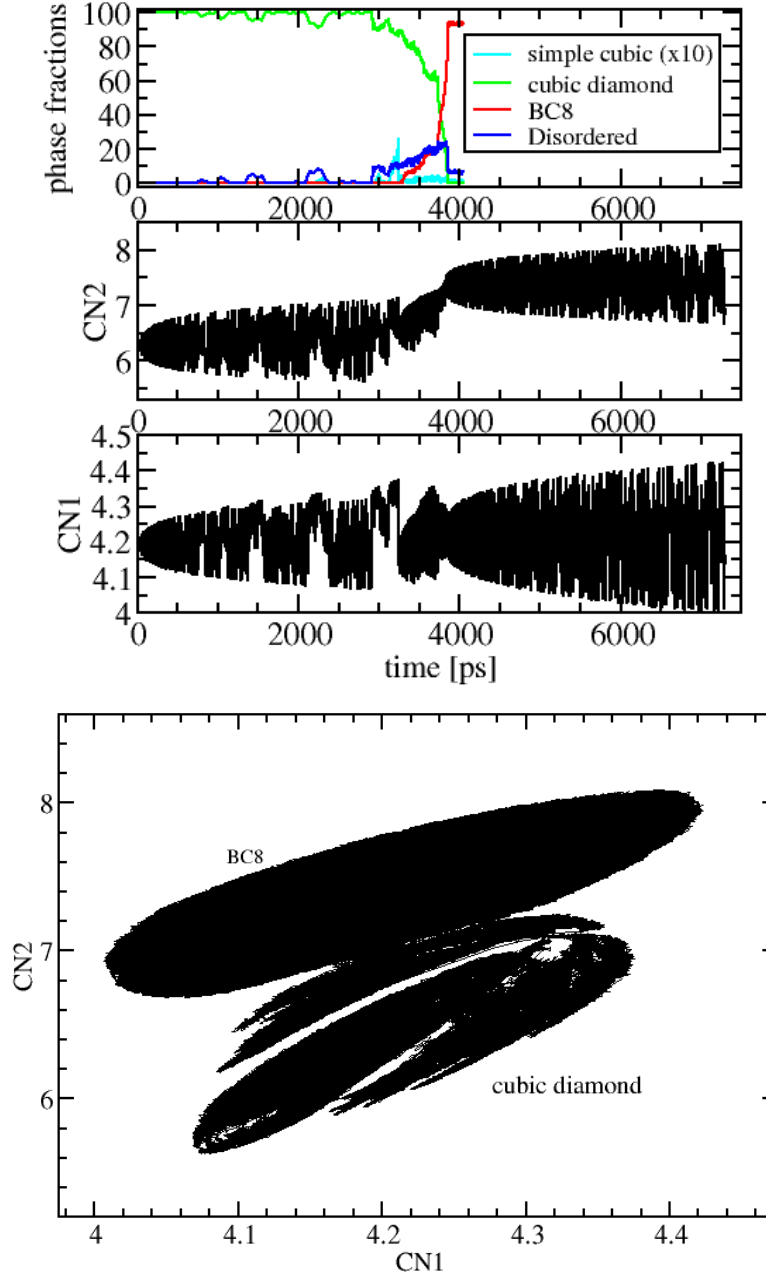

Fig.S3 Upper panel: time evolution of the collective variables  $CN1$  and  $CN2$  and phase fractions. The fraction of the simple cubic phase was multiplied by 10 for better readability. Lower panel: Space of the CVs explored by metadynamics.

# Transition from cubic diamond to simple cubic, 2.1 TPa and 4000 K

4096 atoms

Metadynamics parameters

CN1:  $D_0 = 0.09$  nm,  $R_0 = 0.05$  nm,  $\sigma = 0.02$

CN2:  $D_0 = 0.12$  nm,  $R_0 = 0.05$  nm,  $\sigma = 0.05$

$W = 300$  kJ/mol,  $PACE = 1000$

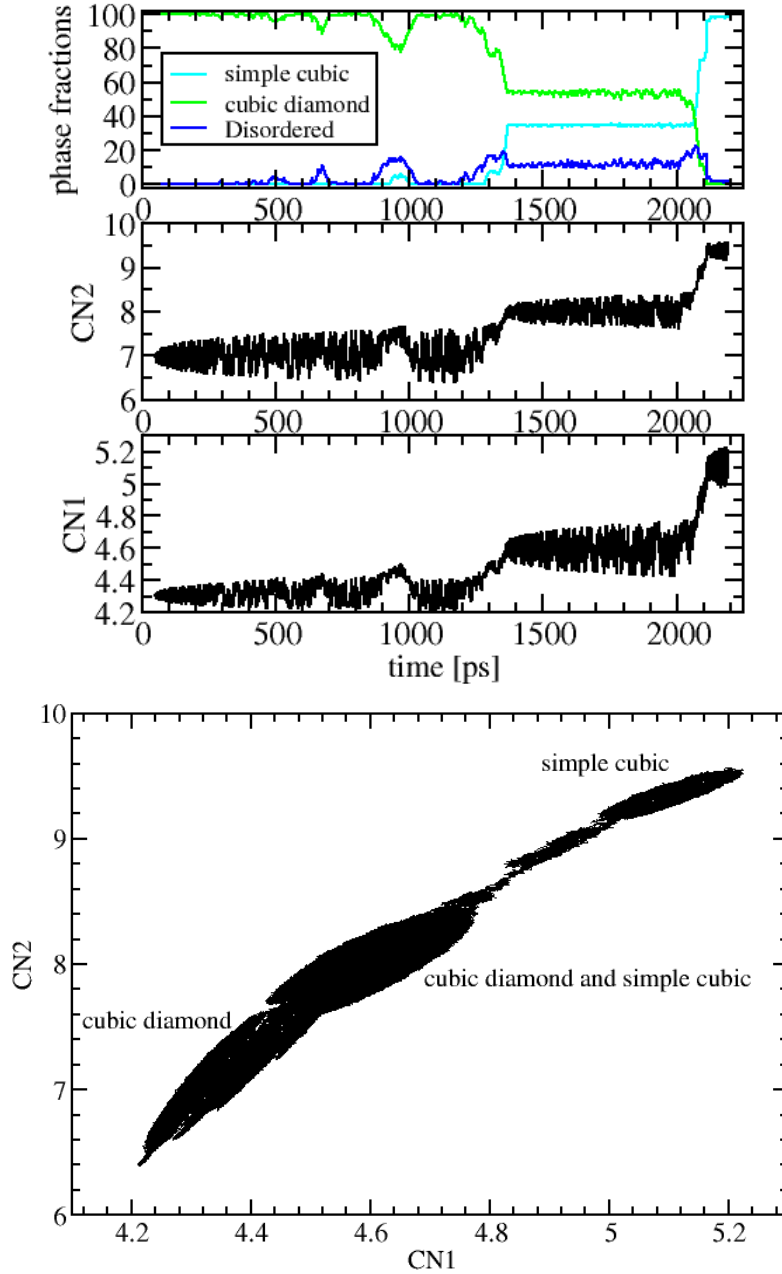

Fig.S4 Upper panel: time evolution of the collective variables  $CN1$  and  $CN2$  and phase fractions. Lower panel: Space of the CVs explored by metadynamics.

# Transition from hexagonal diamond to BC8, 1.8 TPa and 4000 K

4608 atoms

Metadynamics parameters

CN1:  $D_0 = 0.09$  nm,  $R_0 = 0.05$  nm,  $\sigma = 0.01$

CN2:  $D_0 = 0.12$  nm,  $R_0 = 0.05$  nm,  $\sigma = 0.05$

$W = 300$  kJ/mol,  $PACE = 1000$

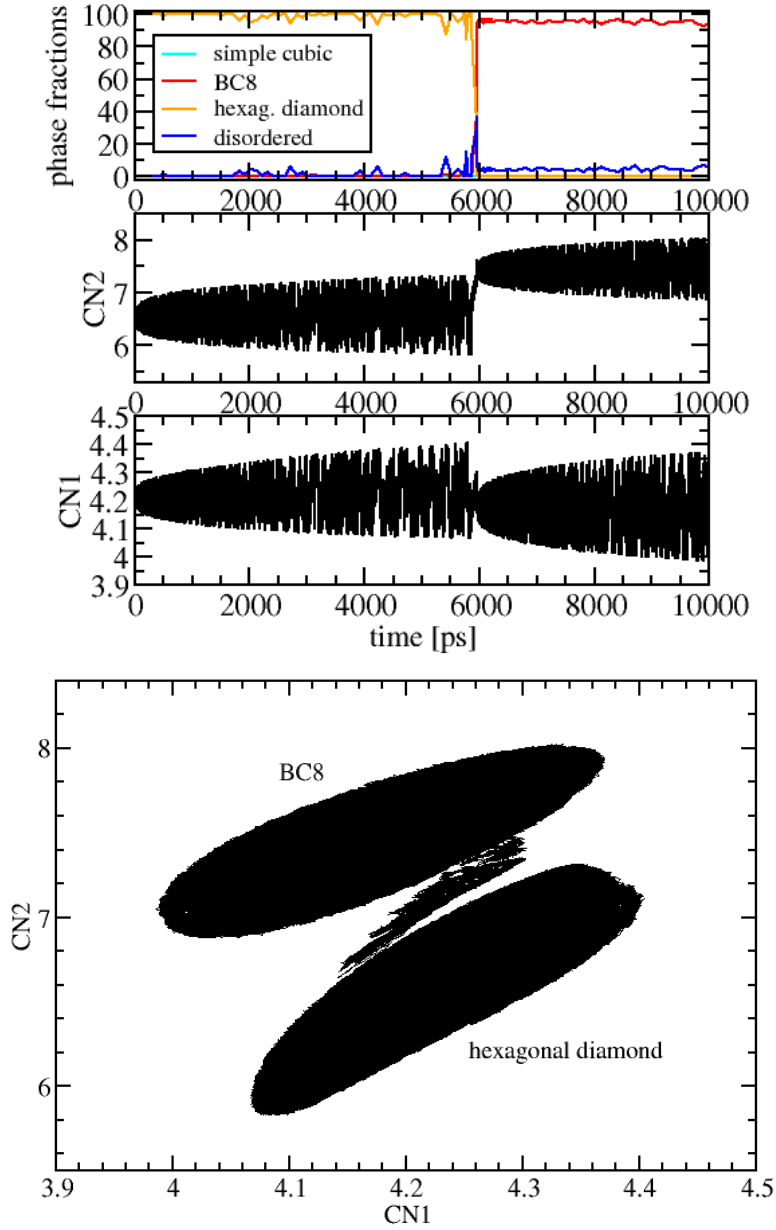

Fig.S5 Upper panel: time evolution of the collective variables  $CN1$  and  $CN2$  and phase fractions. Lower panel: Space of the CVs explored by metadynamics.

## Transition from simple cubic to BC8, 1.5 TPa and 3500 K

4096 atoms

Metadynamics parameters

$CN1$ :  $D_0 = 0.09$  nm,  $R_0 = 0.05$  nm,  $\sigma = 0.02$

$CN2$ :  $D_0 = 0.12$  nm,  $R_0 = 0.05$  nm,  $\sigma = 0.05$

$W = 300$  kJ/mol,  $PACE = 1000$

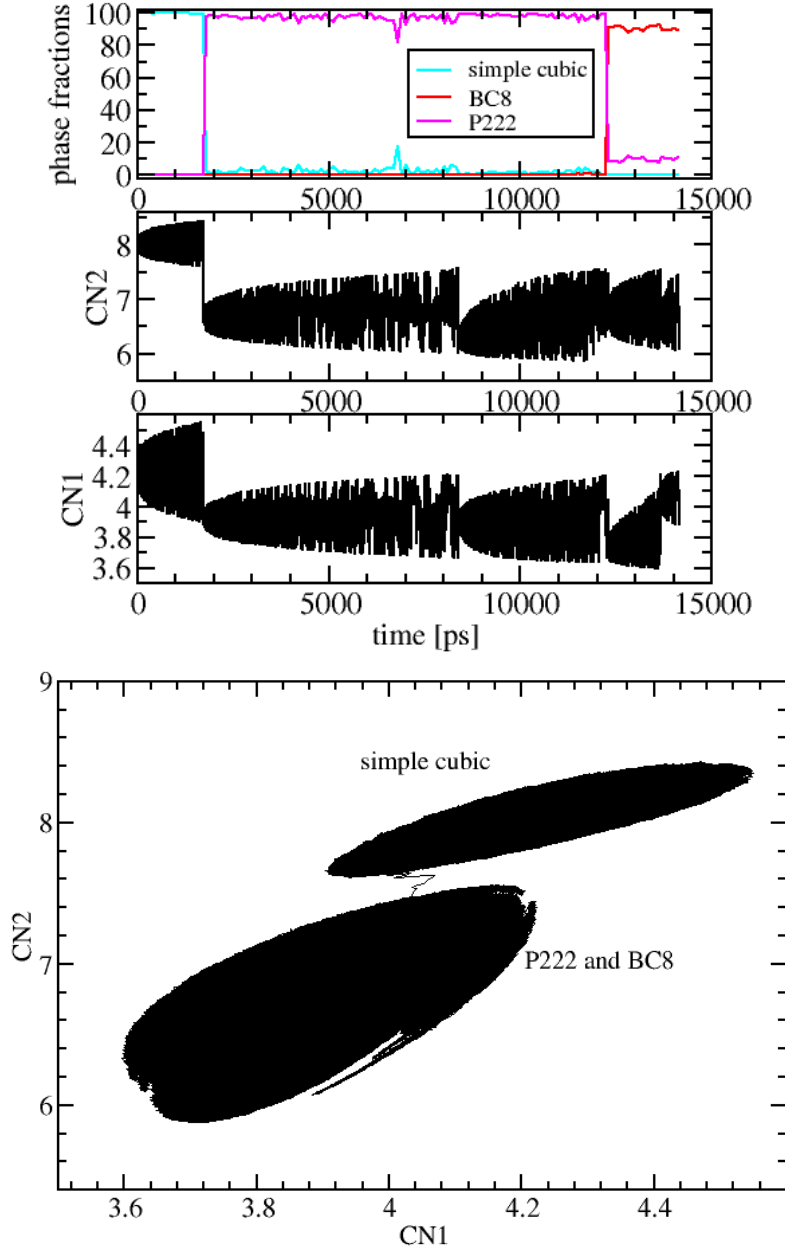

Fig.S6 Upper panel: time evolution of the collective variables  $CN1$  and  $CN2$  and phase fractions. Lower panel: Space of the CVs explored by metadynamics.

# Transition from BC8 to cubic diamond/hexagonal diamond, 200 GPa and 3000 K

1024 atoms

CN1:  $D_0 = 0.085$  nm,  $R_0 = 0.05$  nm,  $\sigma = 0.05$

CN2:  $D_0 = 0.14$  nm,  $R_0 = 0.06$  nm,  $\sigma = 0.05$

$W = 80$  kJ/mol,  $PACE = 1000$

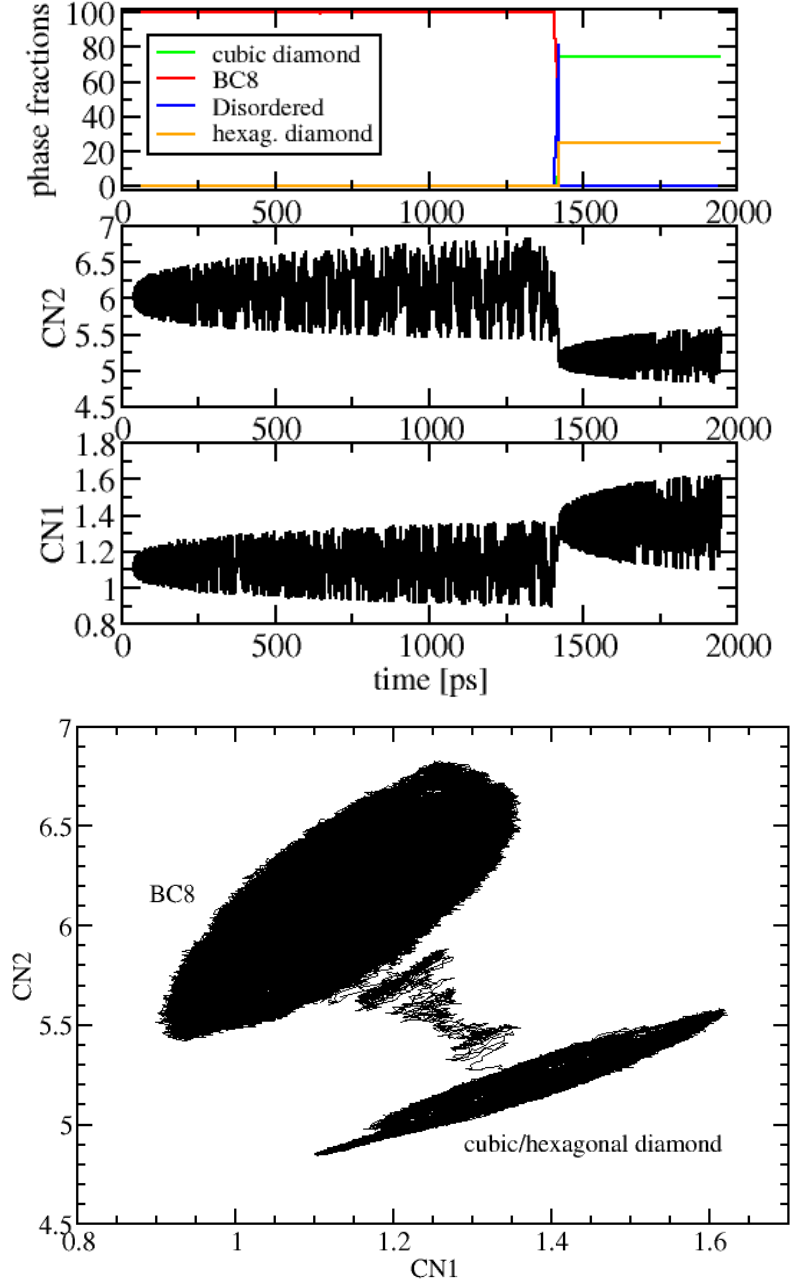

Fig.S7 Upper panel: time evolution of the collective variables  $CN1$  and  $CN2$  and phase fractions. Lower panel: Space of the CVs explored by metadynamics.



## Properties of the $P222$ phase

The structure is orthorhombic, space group 16,  $P222$  with lattice parameters  $a = 1.98637$  Å,  $b = 2.19273$  Å,  $c = 8.98310$  Å. The unit cell contains 16 atoms on Wyckoff 4u positions (0.75223, 0.65534, 0.28239), (0.74134, 0.84485, 0.40781), (0.25398, 0.66689, 0.09524), 2r positions (0.50000, 0.00000, 0.19045), 1a position (0., 0., 0.) and 1g position (0., 0.5, 0.5). In Fig.S8 we show the view of the structure along the  $a$  and  $b$  axis. In Fig.S9 we show the enthalpy of this phase compared to cubic diamond, BC8 and simple cubic. Interestingly, the enthalpy of the  $P222$  becomes at 1.8 TPa lower than that of the cubic diamond while being above that of BC8 in the whole interval between 1 and 3 TPa.

The figure Fig.S9 shows also the electronic density of states calculated at 1.5 TPa. The density of states has at the Fermi energy a very small gap suggesting the phase is nearly semi-metallic. Since the PBE functional employed [S4] is known to underestimate the band gap, in reality the system is likely to be a small gap semiconductor. The *ab initio* calculations were performed by the VASP package [S5–S8] using the C\_h pseudopotential with a cutoff of 910 eV and a Monkhorst-Pack [S9] grid of k-points  $8 \times 8 \times 8$  for the cubic diamond and BC8 phases,  $8 \times 8 \times 2$  for the  $P222$  phase and  $16 \times 16 \times 16$  for the simple cubic phase.

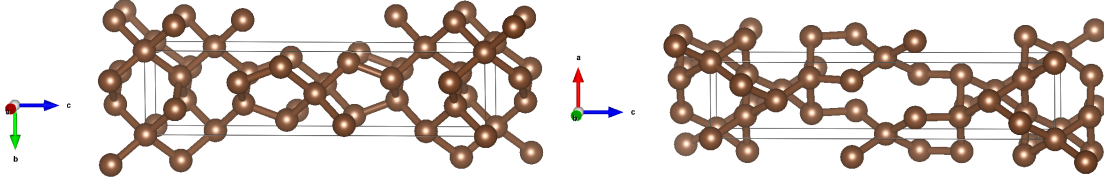

Fig.S8 Left panel: The  $P222$  viewed along the  $a$  axis. Right panel: The  $P222$  viewed along the  $b$  axis. The figures were prepared using the VESTA package [S10].

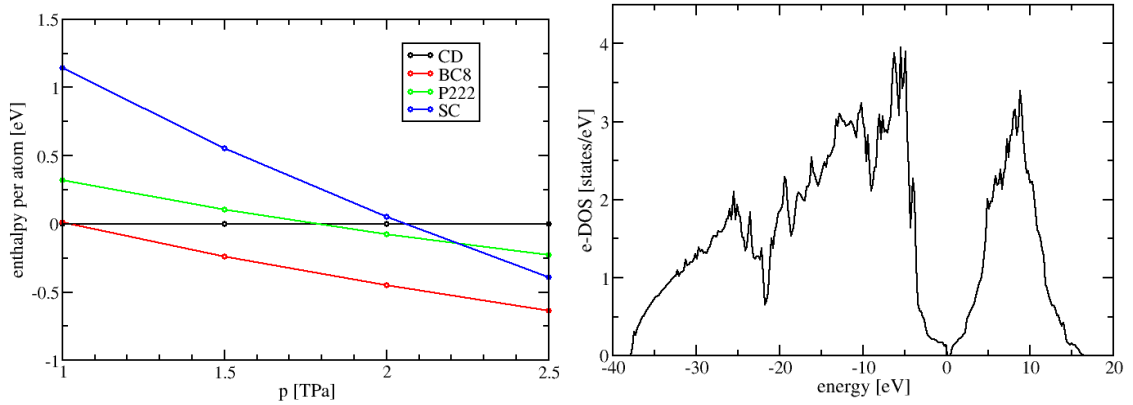

Fig.S9 Left panel: Enthalpies of the four phases with respect to the cubic diamond phase as function of pressure. Right panel: Electronic density of states of the  $P222$  phase at 1.5 TPa, the Fermi energy is located at zero.

## Pressure dependence of the barrier for transformation of BC8 to cd/hd at 3000 K

The barriers were determined in a simple manner from the depth of the initial free-energy well at the moment of the transition to a different state. We did not perform a finite-size scaling analysis to determine the convergence to the thermodynamic limit and therefore the values are representative only for the specific system size. Nevertheless, the temperature and pressure dependence of the barrier height for the same system size provides a useful information.

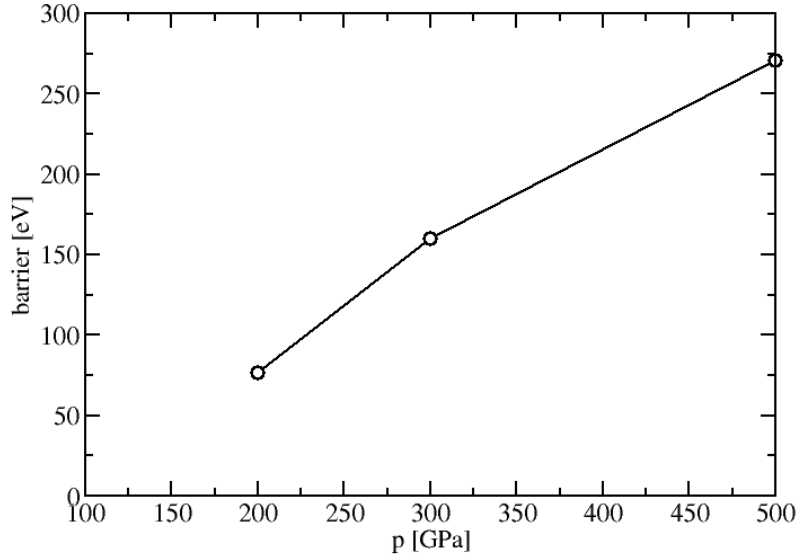

Fig.S10 Barrier for the transformation of BC8 to cd/hd as function of pressure at 3000 K, system contains 1024 atoms.

## Algorithm for identification of crystalline phases

The structural state of the atoms was determined using two complementary approaches: the Polyhedral Template Matching (PTM) method (which identified cubic and hexagonal diamond), and the Machine Learning Structure Identification (MLSI) method [S11], both implemented within the OVITO package [S12]. The MLSI framework was specifically trained in the pressure–temperature region of interest to ensure robust classification. In particular, training of the BC8 phase was performed on nearly defect-free BC8 configurations sampled along the melting line, including structures equilibrated at temperatures  $\sim 200$  K above and below melting, as well as on a regular temperature-pressure grid extending below the melting point and up to 4000 K. Similarly, training of the  $P222$  phase employed near-ideal  $P222$  reference structures prepared at the conditions corresponding to Fig. 6, supplemented by a systematic grid of training points spanning  $\pm 500$ – $1000$  K in temperature and  $\pm 100$ – $200$  GPa in pressure.

## References

- [S1] Matej Badin and Roman Martoňák. Nucleating a different coordination in a crystal under pressure: A study of the  $b1$ – $b2$  transition in nacl by metadynamics. *Phys. Rev. Lett.*, 127:105701, Aug 2021.
- [S2] Gareth A. Tribello, Massimiliano Bonomi, Davide Branduardi, Carlo Camilloni, and Giovanni Bussi. PLUMED 2: New feathers for an old bird. *Computer Physics Communications*, 185(2):604–613, 2 2014.
- [S3] A. P. Thompson, H. M. Aktulga, R. Berger, D. S. Bolintineanu, W. M. Brown, P. S. Crozier, P. J. in ’t Veld, A. Kohlmeyer, S. G. Moore, T. D. Nguyen, R. Shan, M. J. Stevens, J. Tranchida, C. Trott, and S. J. Plimpton. LAMMPS - a flexible simulation tool for particle-based materials modeling at the atomic, meso, and continuum scales. *Comp. Phys. Comm.*, 271:108171, 2022.
- [S4] John P. Perdew, Kieron Burke, and Matthias Ernzerhof. Generalized gradient approximation made simple. *Phys. Rev. Lett.*, 77:3865–3868, Oct 1996.
- [S5] G. Kresse and J. Hafner. Ab initio molecular dynamics for liquid metals. *Phys. Rev. B*, 47:558–561, Jan 1993.
- [S6] G. Kresse and J. Furthmüller. Efficient iterative schemes for ab initio total-energy calculations using a plane-wave basis set. *Phys. Rev. B*, 54:11169–11186, Oct 1996.
- [S7] G. Kresse and J. Furthmüller. Efficiency of ab-initio total energy calculations for metals and semiconductors using a plane-wave basis set. *Computational Materials Science*, 6(1):15–50, 1996.
- [S8] G. Kresse and D. Joubert. From ultrasoft pseudopotentials to the projector augmented-wave method. *Phys. Rev. B*, 59:1758–1775, Jan 1999.
- [S9] Hendrik J. Monkhorst and James D. Pack. Special points for brillouin-zone integrations. *Phys. Rev. B*, 13:5188–5192, Jun 1976.
- [S10] Koichi Momma and Fujio Izumi. VESTA3 for three-dimensional visualization of crystal, volumetric and morphology data. *Journal of Applied Crystallography*, 44(6):1272–1276, Dec 2011.

- [S11] Linus C Erhard, Daniel Utt, Arne J Klomp, and Karsten Albe. Crystal structure identification with 3d convolutional neural networks with application to high-pressure phase transitions in sio<sub>2</sub>. *Modelling and Simulation in Materials Science and Engineering*, 32(6):065029, aug 2024.
- [S12] Alexander Stukowski. Visualization and analysis of atomistic simulation data with ovito—the open visualization tool. *Modelling and Simulation in Materials Science and Engineering*, 18(1):015012, dec 2009.
